# Supplementary material for: Dynamic Recompilation of Software Network Services with Morpheus
Source: arXiv:2106.08833 source file (2021-06-16)
Supplement: Supplementary file 1 [file appendix.tex]

\section{Other tests}

\begin{table*}[!htbp]
\centering
\begin{tabular}{|l|c|c|c|c|c|c|c|c|c|}
\hline
\multicolumn{1}{|c|}{\multirow{2}{*}{\textbf{Application}}} & \multicolumn{3}{c|}{High locality} & \multicolumn{3}{c|}{Low locality} & \multicolumn{3}{c|}{No locality} \\ \cline{2-10} 
\multicolumn{1}{|c|}{}                             & Baseline   & Morpheus   & Gain     & Baseline   & Morpheus  & Gain     & Baseline  & Morpheus  & Gain     \\ \hline
L2 Switch                                          & 2.89       & 4.43       & 53.52\%  & 2.89       & 3.35      & 15.74\%  & 2.79      & 3.11      & 11.65\%  \\ \hline
Router                                             & 2.70       & 5.25       & 94.01\%  & 2.70       & 4.77      & 76.21\%  & 2.70      & 2.92      & 7.86\%   \\ \hline
NAT                                                & 4.36       & 4.58       & +5.15\%  & 4.28       & 4.21      & -6.46\%  & 4.07      & 3.66      & -10.02\% \\ \hline
BPF-iptables                                       & 1.31       & 1.77       & 34.52\%  & 1.21       & 1.58      & 29.88\%  & 1.20      & 1.56      & 29.23\%  \\ \hline
Katran                                             & 4.09       & 5.14       & 25.65\%  & 4.09       & 4.72      & 15.51\%         & 4.09      & 4.22      & 3.39\%    \\ \hline
OvS-eBPF                                           &            &            &          &            &           &          &           &           &          \\ \hline
\end{tabular}
\caption{Single-core throughput (Mpps) with 64B packets for various eBPF-based NFs with the \fname compiler depending on different traffic patterns} \label{tab:three_tables}
\end{table*}

\begin{table*}[!htbp]
\small
\centering
\begin{tabular}{|l|c|l|l|c|l|l|c|l|l|c|l|l|c|l|l|c|l|l|}
\hline
\multicolumn{1}{|c|}{\multirow{2}{*}{Application}} & \multicolumn{3}{c|}{Cycles}            & \multicolumn{3}{c|}{Instructions}        & \multicolumn{3}{c|}{Cache reference} & \multicolumn{3}{c|}{Cache misses}    & \multicolumn{3}{c|}{Branches}          & \multicolumn{3}{c|}{LLC-load-miss}   \\ \cline{2-19} 
\multicolumn{1}{|c|}{}                             & \multicolumn{3}{c|}{Base/Morp/Gain}    & \multicolumn{3}{c|}{Base/Morp/Gain}      & \multicolumn{3}{c|}{Base/Morp/Gain}  & \multicolumn{3}{c|}{Base/Morp/Gain}  & \multicolumn{3}{c|}{Base/Morp/Gain}    & \multicolumn{3}{c|}{Base/Morp/Gain}  \\ \hline
L2 Switch                                          & \multicolumn{3}{c|}{999.4/651/-35\%}   & \multicolumn{3}{c|}{2648.3/1446.7/-45\%} & \multicolumn{3}{c|}{2.81/3.06/+9\%}  & \multicolumn{3}{c|}{0.1/0.08/-21\%}  & \multicolumn{3}{c|}{473.6/212.3/-55\%} & \multicolumn{3}{c|}{0.1/0.08/-21\%}  \\ \hline
Router                                             & \multicolumn{3}{c|}{1021.4/549/-46\%}  & \multicolumn{3}{c|}{2510.5/1238.9/-51\%} & \multicolumn{3}{c|}{3.43/3.59/+5\%}  & \multicolumn{3}{c|}{0.16/0.01/-96\%} & \multicolumn{3}{c|}{401.7/190/-53\%}   & \multicolumn{3}{c|}{0.16/0.01/-96\%} \\ \hline
NAT                                                & \multicolumn{3}{c|}{661/683.1/3\%}     & \multicolumn{3}{c|}{2.51/2.29/-9\%}      & \multicolumn{3}{c|}{3.68/3.59/-2\%}  & \multicolumn{3}{c|}{0.14/0.14/0\%}   & \multicolumn{3}{c|}{294.8/248.7/-16\%} & \multicolumn{3}{c|}{0.14/0.14/0\%}   \\ \hline
BPF-iptables                                       & \multicolumn{3}{c|}{2106.3/1630/-23\%} & \multicolumn{3}{c|}{4188.4/3681.5/-12\%} & \multicolumn{3}{c|}{3.6/3.7/3\%}     & \multicolumn{3}{c|}{0.11/0.11/0\%}   & \multicolumn{3}{c|}{670.3/500.3/-25\%} & \multicolumn{3}{c|}{0.1/0.1/0\%}     \\ \hline
Katran                                             & \multicolumn{3}{c|}{705.9/561.9/-20\%} & \multicolumn{3}{c|}{1729.9/1429.7/-17\%} & \multicolumn{3}{c|}{3.57/3.02/-15\%} & \multicolumn{3}{c|}{0.22/0.01/-95\%} & \multicolumn{3}{c|}{302.3/202.6/-33\%} & \multicolumn{3}{c|}{0.12/0.01/-95\%} \\ \hline
OvS-eBPF                                           & \multicolumn{3}{c|}{}                  & \multicolumn{3}{c|}{}                    & \multicolumn{3}{c|}{}                & \multicolumn{3}{c|}{}                & \multicolumn{3}{c|}{}                  & \multicolumn{3}{c|}{}                \\ \hline
\end{tabular}
\caption{Single core throughput (Mpps) of the various eBPF-based NFs with the \fname compiler.} 
\label{tab:opts-benefits-perf}
\end{table*}

\begin{table*}[!htbp]
\centering
\begin{tabular}{|l|c|c|c|c|c|c|c|}
\hline
\multicolumn{1}{|c|}{\multirow{2}{*}{Application}} & \multicolumn{3}{c|}{Baseline} & \multicolumn{3}{c|}{Morpheus} & \multirow{2}{*}{Gain} \\ \cline{2-7}
\multicolumn{1}{|c|}{}                             & Avg.     & 95\%     & 99\%    & Avg.     & 95\%     & 99\%    &                       \\ \hline
L2 Switch                                          & 175.6    & 185.1    & 186.9   & 137.2    & 144.2    & 145.9   & -28,0\%               \\ \hline
Router                                             & 138.4    & 145.7    & 147.3   & 13.7     & 21.6     & 36.8    & -911\%                \\ \hline
NAT                                                & 13.5     & 20.1     & 33.1    & 13.6     & 21.9     & 38.4    & +0.73\%               \\ \hline
BPF-iptables                                       & 374.4    & 392.5    & 398.9   & 266.0    & 282.8    & 287.1   & -40.7\%               \\ \hline
Katran                                             & 43.1     & 60.9     & 65.7    & 37.7     & 57.7     & 62.2    & -12.5\%               \\ \hline
OvS-eBPF                                           &          &          &         &          &          &         &                       \\ \hline
\end{tabular}
\caption{Latency ($\mu$sec) of the various eBPF-based NFs with the \fname compiler.} 
\label{fig:opts-benefits-latency}
\end{table*}
